# Supplementary material for: Enumerating Error Bounded Polytime Algorithms Through Arithmetical Theories
Source: arXiv:2311.15003 source file (2023-11-25)
Supplement: Supplementary file 1 [file appendix.tex]

\section{Proofs from Section~\ref{sec4.1}}

\subsection{Proof of Theorem~\ref{thm:RStoPOR}$(\Leftarrow)$}
In order to prove Theorem~\ref{thm:RStoPOR}($\Leftarrow$),
%we 
%need to introduce the following convention:
%every string $s\in \Ss$ can be seen as a term $\overline{s}\in\Lpw$,
%such that $\overline{\eepsilon}=\epsilon$,
%$\overline{s\zzero}=\overline{s}  \zero$
%and $\overline{s\oone}=\overline{s} \one$.
%%
%Moreover, 
we introduce a slightly-modified version
of Parikh's theorem~\cite{Parikh},
which is usually presented
in the context of Buss' bounded arithmetics,
as stating that given a Boolean formula $F$
(in $\mathcal{L}_{\mathbb{N}}$)
such that $S^i_2 \vdash \forall \vec{x}.\exists y.B(\vec{x},y)$,
then there is a term $t(\vec{x})$ such that
$S^i_2 \vdash \forall \vec{x}.\exists y\preceq
t(\vec{x}).B(\vec{x},y)$~\cite{Buss98}.

\begin{prop}\label{prop:Parikh}
Let $F(\vec{x},y)$ be a bounded formula in
$\Lpw$ such that $\RS\vdash (\forall\vec{x})(\exists y)F(\vec{x},y)$.
Then, there is a term $t$ such that
$\RS\vdash \forall \vec{x}.\exists y \preceq t(\vec{x}).F(\vec{x},y)$.
\end{prop}

\begin{proof}[Proof of Theorem~\ref{thm:RStoPOR}($\Leftarrow$)]
The proof is by induction on the structure of functions in $\POR$.
We consider the query function only as all other cases are standard.
$f=\query$ is $\Sigma^b_1$-representable
in $\RS$ by  the formula
$$
G_{\query}(x,y) := \big(\Flip(x) \wedge y=\one\big) \vee
\big(\neg \Flip(x) \wedge y=\zero\big).
$$
Notice that the proof relies on the fact that every
$f\in\POR$ invokes \emph{exactly one} oracle.
\begin{enumerate}
\itemsep0em

\item Existence is proved by cases.
Intuitively if $\RS\vdash \Flip(x)$, we let $y=\one$.
By the reflexivity of identity $\RS\vdash \one=\one$ holds,
so $\RS \vdash \Flip(x)\wedge \one=\one$.
Then, we conclude by purely-logical rules
$\RS \vdash \exists y.(\Flip(x)\wedge \one=\one) \vee
(\neg \Flip(x) \wedge \one=\zero)$.
If $\RS\vdash \neg \Flip(x)$, we let $y=\zero$ and
proceed int he same way.

\item Uniqueness is established relying on the transitivity of identity.

\item For every $n,m\in \Ss$
and $\omega^* \in \Os$,
$\query(n,\omega^*)=m$ iff $\omega^*\in
\model{G_{\query}(\overline{n}, \overline{m})}$.
Assume $m=\oone$. Then $\query(n,\omega^*)=\oone$,
i.e.~$\omega^*(n)=\oone$,
\small
\begin{align*}
\model{(\Flip(\overline{n}) \wedge \overline{m}=\one) \vee
(\neg \Flip(\overline{n}) \wedge \overline{m}=\zero)} &=
\model{\Flip(\overline{n})\wedge \overline{m}=\one} \cup
\model{\neg \Flip(\overline{n}) \wedge \overline{m}=\zero} \\
&= (\model{\Flip(\overline{n})} \cap \model{\one=\one})
\cup (\model{\neg\Flip(\overline{n})} \cap \model{\one=\zero}) \\
&= (\model{\Flip(\overline{n})}\cap \model{\one=\one})
\cup (\model{\neg\Flip(\overline{n})} \cap \emptyset) \\
&=  \model{\Flip(n)} \\
&= \{\omega \ | \ \omega(n)=\oone\}.
\end{align*}
\normalsize
Clearly, $\omega^* \in
\model{(\Flip(\overline{n}) \wedge \overline{m}=\one)
\vee
(\neg\Flip(\overline{n}) \wedge \overline{m}=\zero)}$.
The case $m=\zzero$ and the opposite direction
are proved in a similar way.
\end{enumerate}

Inductive cases are also standard.
For bounded recursion the proof is
especially convoluted, following~\cite{Ferreira88}.
\end{proof}

\subsection{Proof of Theorem~\ref{thm:RStoPOR}$(\Rightarrow)$}

The proof of Theorem~\ref{thm:RStoPOR}$(\Rightarrow)$
adapts the strategy used by Cook and Urquhart for IPV$^{\omega}$~\cite{CookUrquhart} and is structured as follows:
\begin{enumerate}
\itemsep0em
\item We introduce a basic equational theory $\POR^\lambda$ for a simply
typed $\lambda$-calculus with primitives corresponding to functions of $\POR$.

\item We define the \emph{intuitionistic} theory $I\POR^\lambda$,
extending $\POR^\lambda$ with usual predicate calculus and
an $\NP$-induction schema, and
$I\RS$, which is the intuitionistic version of $\RS$.
We show $I\POR^\lambda$ able to prove all theorems of $I\RS$.

\item We develop a realizability interpretation of $I\POR^\lambda$
(inside itself): for any derivation of
$\forall x.\exists y.A(x,y)$, with $A \in \Sigma^b_0$,
a $\lambda$-term $\tTerm$ of $\POR^\lambda$ can be extract,
such that $\vdash_{I\POR^\lambda} \forall x.A(x,\tTerm)$.
We show that every function which is $\Sigma^b_1$-representable
in $I\RS$ is in $\POR$.

\item Finally, we extend this result to classical $\RS$,
showing that any $\Sigma^b_1$-formula provable in $I\POR^\lambda$
+ Excluded Middle (EM, for short) is already provable in $I\POR^\lambda$.
\end{enumerate}

%%%%% The Theory POR^\lambda
\paragraph*{The Theory $\POR^\lambda$}
$\POR^\lambda$ is an equational theory for a simply
typed $\lambda$-calculus augmented with primitives
for functions of $\POR$.
Actually, these do not exactly correspond to basic functions
in $\POR$, although the resulting function algebra
is proved equivalent.
%In particular, in $\POR^\lambda$ defining equations for functions different from the recursion operator should not depend  on it and on functions defined without it.

Types of $\POR^\lambda$ are standard,
while terms are obtained by adding to simply
typed $\lambda$-terms constants from the signature below:
\footnotesize
\begin{align*}
\zeroT, \oneT, \epsilonT &: \sType \\
\Tail, \Flipcoin &: \sType \arrowT \sType \\
\circ, \Trunc &: \sType \arrowT \sType \arrowT \sType \\
\Cond &: \sType \arrowT \sType \arrowT \sType \arrowT \sType \arrowT
\sType \\
\Rec &: \sType \arrowT (\sType \arrowT \sType \arrowT \sType)
\arrowT (\sType \arrowT \sType \arrowT \sType)
\arrowT (\sType \arrowT \sType) \arrowT \sType \arrowT \sType.
\end{align*}
\normalsize
Intuitively, $\Tail(x)$ computes the string obtained by deleting the
first digit of $x$,
$\Trunc(x,y)$ that obtained by truncating $x$ at the length
of $y$,
$\Cond(x,y,z,w)$ the function that yields $y$ if $x=\eepsilon$,
$z$ if $x=x'\zzero$ and $w$ if $x=x'\oone$,
$\Flipcoin(x)$ indicates a random $\zzero$/$\oone$ generator,
and $\Rec$ is the operator for bounded recursion on notation.

\begin{notation}
In the following, we often define terms implicitly using bounded recursion
on notation.
We now introduce a few abbreviations for composed functions:
\begin{itemize}
\itemsep0em
\item $\BT(x) := \Cond(x,\epsilonT, \zeroT,\oneT)$
indicates the function computing the last digit of $x$.
%i.e. coerces $x$ to a Boolean value.

\item $\BNeg(x) := \Cond(x,\epsilonT, \oneT,\zeroT)$
computes the Boolean negation of $\BT(x)$.

\item $\BOr(x,y) := \Cond(\BT(x), \BT(y), \BT(y), \zeroT)$
coerces $x,y$ to Booleans and performs OR-operation.

\item $\BAnd(x,y) :=\Cond(\BT(x), \epsilonT, \zeroT, \BT(y))$
coerces $x,y$ to Booleans and performs AND-operation.

\item $\Eps(x) := \Cond(x,\oneT,\zeroT,\zeroT)$ indicates
the characteristic function of ``$x = \epsilon$''.

\item $\BoolT(x) := \BAnd(\Eps(\Tail(x)), \BNeg(\Eps(x)))$
is the characteristic function of ``$x = \zero \vee x=\one$''.

\item $\Zero(x) := \Cond(\BoolT(x), \zeroT, \Cond(x,\zeroT,\zeroT,\oneT),\zeroT)$
is the characteristic function of the predicate ``$x = \zero$''.

\item $\Conc(x,y)$ indicates the concatenation function.
%defined as:
%\begin{align*}
%\Conc(x,\epsilonT) &:= x \\
%\Conc(x,y\zeroT) &:= \Conc(x,y)\zeroT \\
%\Conc(x,y\oneT) &:= \Conc(x,y)\oneT.
%\end{align*}

\item $\Eq(x,y)$ is the characteristic function of
``$x = y$'' and is defined by double recursion.

\item  $\Times(x,y)$ is the function for self-concatenation,
$x,y\mapsto x\times y$.

\item $\Sub(x,y)$ is the initial-substring function $x,y\mapsto S(x,y)$.
\end{itemize}
\end{notation}

$\POR^\lambda$ is reminiscent of PV$^\omega$~\cite{CookUrquhart}
(without the induction rule R5),
the main difference being the constant $\Flipcoin$,
denoting a function which randomly generates
either $\zzero$ or $\oone$.
Formulas of $\POR^\lambda$ are all equations
$\tTerm = \uTerm$, where $\tTerm,\uTerm$ are terms of type $\sType$.

\begin{defn}[The Theory $\POR^\lambda$]
Axioms of $\POR^\lambda$ are the following ones:
\begin{itemize}
\itemsep0em
\item Defining axioms for the constants of $\POR^\lambda$
%\footnotesize
\begin{align*}
\epsilonT x = x\epsilonT &= x \\
x(y\boolT) &= (xy)\boolT \\
\\
\Tail(\epsilonT) &= \epsilonT \\
\Tail(x\boolT) &= x \\
\\
\Trunc(x,\epsilonT) = \Trunc(\epsilonT,x) &= \epsilonT \\
\Trunc(x\boolT,y\zeroT)= \Trunc(x\boolT, y\oneT) &= \Trunc(x,y)\boolT \\
\\
\Cond(\epsilonT, y, z, w) &= y \\
\Cond(x\zeroT, y, z,w) &= z \\
\Cond(x\oneT, y,z,w) &= w \\
\\
\BoolT(\Flipcoin(x)) &= \oneT \\
\\
\Rec(x,h_0,h_1,k,\epsilonT) &= x \\
\Rec(x,h_0,h_1,k,y\zeroT) &= \Trunc(h_0y(\Rec(x,h_0,h_1,k,y)),
ky) \\
\Rec(x,h_0,h_1,k,y\oneT) &=
\Trunc(h_1y(\Rec(x,h_0,h_1,k,y)),ky),
\end{align*}
\normalsize
with $\boolT\in\{\zeroT,\oneT\}$.

\item The $(\beta)$- and $(\nu)$-axioms:
%\footnotesize
\begin{align}
\mathsf{C}\big[(\lambda x.\tTerm)\uTerm\big] &=
\mathsf{C}\big[\tTerm\{\uTerm/x\}\big]  \ \ \
\tag{$\beta$} \\
\mathsf{C}\big[\lambda x.\tTerm x\big] &=
\mathsf{C}[\tTerm] \ \ \
\tag{$\nu$}
\end{align}
\normalsize
where $\mathsf{C}\big[\cdot\big]$ indicates
a context with a unique occurrence of the hole
$\big[ \ \big]$, so that $\mathsf{C}\big[\tTerm\big]$
denotes the variable-capturing replacement of
$\big[ \ \big]$ by $\tTerm$ in $\mathsf{C}\big[ \ \big]$.
\end{itemize}
\normalsize
Inference rules of $\POR^\lambda$ are the following ones:
%\footnotesize
\begin{align}
\tTerm = \uTerm &\vdash \uTerm = \tTerm
\tag{R1} \\
\tTerm = \uTerm, \uTerm = \vTerm &\vdash \tTerm = \vTerm   \tag{R2} \\
\tTerm = \uTerm &\vdash \vTerm\{\tTerm/x\} = \vTerm\{\uTerm/x\} \tag{R3} \\
\tTerm = \uTerm &\vdash  \tTerm\{\vTerm/x\} = \uTerm\{\vTerm/x\}. \tag{R4}
\end{align}
\end{defn}
\normalsize
Let $\vdash_{\POR^\lambda} \tTerm = \uTerm$
indicate that the equation $\tTerm=\uTerm$
is deducible by instances of axioms
and inference rules above.
Given a set of equations $T$,
$T\vdash_{\POR^\lambda}\tTerm=\uTerm$
indicates that $\tTerm=\uTerm$ is deducible using
the given axioms and rules plus equations from $T$.

For any string $s\in \Ss$ and $\omega\in\Os$,
$\ooverline{s}:\sType$
denotes the term of $\POR^\lambda$ corresponding
to it, i.e.~$\ooverline{\eepsilon} = \epsilonT,
\ooverline{s\zzero}=\ooverline{s}\zeroT$,
$\ooverline{s\oneT} = \ooverline{s}\oneT$,
and $T_\omega$
is the set of all equations of the form
$\Flipcoin(\ooverline{s})=\ooverline{\omega(s)}$.

\begin{defn}[Provable Representability]
Let $f:\Os \times \Ss^k \rightarrow \Ss$.
A term $\tTerm : \sType \arrowT \dots \arrowT \sType$
of $\POR^\lambda$ \emph{provably represents f}
when for all strings $s_1,\dots, s_j,s\in \Ss$ and
$\omega\in \Os$,
$$
f(s_1,\dots, s_n,\omega)=s \Leftrightarrow T_\omega
\vdash_{\POR^\lambda} \tTerm \ooverline{s_1}
\dots \ooverline{s_j} = \ooverline{s}.
$$
\end{defn}

\begin{ex}
The term $\Flipcoin: \sType \arrowT \sType$
provably represents the query function $\query(x,\omega)=
\omega(x)$ of $\POR$.
Indeed, for any $s\in \Ss$ and
$\omega \in \Os$,
$\Flipcoin(\ooverline{s})=\ooverline{\omega(s)}
\vdash_{\POR^\lambda} \Flipcoin(\ooverline{s})=
\ooverline{\query(s,\omega)}$.
\end{ex}
%
%
%
%Some of the terms described above provably represent the intended functions.
Notice that terms $\Tail, \Trunc, \Cond$ provably
represents $f_{\Tail}, f_{\Trunc}$ and $\Cond$, resp.,
where $f_{\Tail}(s,\omega)$ is the string obtained by
chopping the first digit
of $s$
%(with $E(s,\omega)=\eepsilon$)
and $f_{\Trunc}(s_1,s_2,\omega)=s_1|_{s_2}$.

%\begin{lemma}
%Terms $\Tail, \Trunc, \Cond$ provably represent $f_{\Tail}, f_{\Trunc}$ and $\Cond$, resp.
%\end{lemma}

\begin{theorem}\label{theorem1}
\begin{enumerate}
\itemsep0em
\item Any function $f\in \POR$ is provably represented
by a term $\tTerm\in \POR^\lambda$.

\item For any $\tTerm\in \POR^\lambda$,
there is an $f\in\POR$ such that $f$
is provably represented by $\tTerm$.
\end{enumerate}
\end{theorem}
\begin{proof}[Proof Sketch]
$(\Rightarrow)$ The proof is by induction on the structure
of $f\in \POR$. \\
$(\Leftarrow)$ As a consequence of the normalization,
a $\beta$-normal term $\tTerm: \sType \arrowT \dots \arrowT \sType$
cannot contain variables of higher types
and each possible normal form represents
functions in $\POR$.
\end{proof}

\begin{cor}
For any function $f:\Ss^j \times \Os \rightarrow \Ss$,
$f\in \POR$ when $f$ is provably represented by some
$\tTerm:\sType \arrowT \dots \arrowT \sType \in \POR^\lambda$.
\end{cor}

\paragraph*{The Theory $I\POR^\lambda$}

The theory $\POR^\lambda$ is rather weak,
as, for example, one cannot prove even simple
equations as $x=\Tail(x)\BT(x)$
(as some form of induction is needed).
So, we introduce $I\POR^\lambda$,
which extends $\POR^\lambda$ with basic predicate calculus
and a restricted induction principle.
We also define the intuitionistic version of $\RS$,
the so-called $I\RS$.
We show that all theorems of $\POR^\lambda$ and $I\RS$
are provable in $I\POR^\lambda$
and
the latter provides a language
to associate derivations in $I\RS$ with
polytime computable functions,
corresponding to $I\POR^\lambda$-terms.

\begin{defn}[Formulas of $I\POR^\lambda$]
(i) All equations
$\tTerm=\uTerm$ of $\POR^\lambda$ are formulas
of $I\POR^\lambda$,
(ii) given (possibly open) term $\tTerm,\uTerm:\sType \in
\POR^\lambda$, $\tTerm\subseteq \uTerm$
and $\Flip(\tTerm)$
are formulas of $I\POR^\lambda$,
(iii) formulas of $I\POR^\lambda$ are closed
under $\wedge,\vee,\rightarrow, \forall,\exists$.
%where $\termT:\sType$ is a possibly open term of $\POR^\lambda$.
\end{defn}
\begin{notation}
We define $\bot := \zeroT = \oneT$ and
$\neg A := A \rightarrow \bot$.
%
%The notion of $\Sigma^b_0$- and $\Sigma^b_1$-formula of $I\POR^\lambda$ is defined as for $\RS$.
Furthermore, any formula of $\RS$ can be seen as a formula
of $I\POR^\lambda$ where each occurrence of
$\zero$ is replaced by $\zeroT$,
$\one$ by $\oneT$,
$\frown$ by $\circ$,
and $\times$ by $\Times$.
In the following, we suppose that any formula of $\RS$
is a formula of $I\POR^\lambda$.
\end{notation}

\begin{defn}[Theory $I\POR^\lambda$]
Axioms and inference rules of $I\POR^\lambda$
include the standard rule of the intuitionistic first-order predicate calculus,
usual rules for equality and the axioms below:
(1) all axioms of $\POR^\lambda$,
(2) $x\subseteq y \leftrightarrow \Sub(x,y)=\oneT$,
(3) $x=\epsilonT \vee x = \Tail(x)\zeroT \vee x=\Tail(x)\oneT$,
(4) $\zeroT = \oneT \rightarrow x=\epsilonT$,
(5) $\Cond(x,y,z,w)=w' \leftrightarrow
(x=\epsilonT \wedge w'=y) \vee
(x=\Tail(x) \zeroT \wedge w'=z) \vee
(x=\Tail(x)\one \wedge w'=w)$,
(6) $\Flip(x) \leftrightarrow \Flipcoin(x)=\oneT$,
(7) Any formula of the form
$(A(\epsilonT) \wedge \forall x.(A(x)\rightarrow
A(x\zeroT)) \wedge
\forall x.(A(x)\rightarrow A(x\oneT))) \rightarrow
\forall y.A(y)$,
where $A$ is of the form $\exists z \preceq \tTerm.
\uTerm=\vTerm$, with $\tTerm$ containing only first-order
open variables.
\end{defn}

\begin{notation}[$\NP$-Predicate]
We will refer to a formula in the form $\exists z\preceq \tTerm.
\uTerm=\vTerm$, with $\tTerm$ containing only
first-order open variables, as an $\NP$-predicate.
\end{notation}

It is now possible to show that all theorems
of both $\POR^\lambda$ and $I\RS$
are derivable in  $I\POR^\lambda$.
In particular, Prop~\ref{prop3}
is proved by systematic inspection of $\POR^\lambda$-rules.

\begin{prop}\label{prop3}
Any theorem of $\POR^\lambda$
is a theorem of $I\POR^\lambda$.
\end{prop}
%\begin{proof}[Proof Sketch]
%By inspecting all rules of $\POR^\lambda$.
%\end{proof}
%
To prove that every theorem of $I\RS$
is derivable in $I\POR^\lambda$
we need to establish a few useful properties concerning
$I\POR^\lambda$.
In particular, the recursion schema of $I\POR^\lambda$
differs from that of $I\RS$ as dealing with formulas
of the form $\exists y\preceq \tTerm.\uTerm=\vTerm$
rather than all the $\Sigma^b_1$-ones.
%
%The two schemas can be related due to  Proposition below, proved by induction on the structurer of formulas.

\begin{prop}\label{prop}
For any $\Sigma^b_0$-formula $A(x_1,\dots, x_n)$
of $\Lpw$,
there is a term $\tTerm_A(x_1,\dots, x_n)$ of $\POR^\lambda$
such that: (i) $\vdash_{I\POR^{\lambda}} A\leftrightarrow
\tTerm_A=\zeroT$, (ii) $\vdash_{I\POR^\lambda}
\tTerm_A = \zeroT \vee \tTerm_A = \oneT$.
\end{prop}
%
%
%
%Results below follows,
%
\begin{cor}\label{cor2}
\begin{itemize}
\item[i.] For any $\Sigma^b_0$-formula $A$,
$\vdash_{I\POR^\lambda} A \vee \neg A$.

\item[ii.] For any closed $\Sigma^b_0$-formula $A$
and $\omega \in \Os$, either
$T_\omega \vdash_{I\POR^\lambda} A$
or $T_\omega \vdash_{I\POR^\lambda} \neg A$.
\end{itemize}
\end{cor}

So we conclude,

\begin{theorem}\label{theorem2}
Any theorem of $I\RS$ is a theorem of $I\POR^\lambda$.
\end{theorem}
\begin{proof}
For any $\Sigma^b_1$-formula
$A=\exists x_1\preceq t_1 \dots \exists x_n\preceq t_n.B$
of $I\RS$,
$\vdash_{I\POR^\lambda}
A \leftrightarrow \exists x_1\preceq \tTerm_1
\dots \exists x_n\preceq \tTerm_n.\tTerm_B = \zeroT$.
So, any instance of the $\Sigma^b_1$-recursion schema
of $I\RS$ is derivable in $I\POR^\lambda$
from the $\NP$-inductions schema.
To prove that $I\POR^\lambda$ extends $I\RS$,
it suffices to check that
all basic axioms of $I\RS$ are provable in $I\POR^\lambda$.
\end{proof}
Furthermore, due to Corollary~\ref{cor2},
we establish Lemma~\ref{lemma13} below.

\begin{lemma}\label{lemma13}
Given a closed $\Sigma^b_0$-formula $A$ in $\Lpw$
and
$\omega \in \Os$,
$T_\omega \vdash_{I\POR^\lambda} A$ iff
$\omega\in \model{A}$.
\end{lemma}

%%%%%% REALIZABILITY
\paragraph*{Realizability}
We introduce realizability as internal to $I\POR^\lambda$
to show that for any derivation in $I\RS$
(actually, in $I\POR^\lambda$) of a formula
$\forall x. \exists y.A(x,y)$,
we extract a functional term $\fTerm: \sType \arrowT \sType$
of $\POR^\lambda$,
such that $\vdash_{I\POR^\lambda} \forall x.A(x,\fTerm x)$.
So, we conclude that if $f$
is $\Sigma^b_1$-representable in $I\RS$, then
$f\in \POR$.

\begin{notation}
Let $\mathbf{x},\mathbf{y}$ denote finite sequences of term
variables, $\mathbf{x}(\mathbf{y})$ be an abbreviation
for $y_1(\mathbf{x}), \dots, y_k(\mathbf{x})$.
Let  $\Lambda$ be a shorthand for the empty sequence and
$y(\Lambda):=y$.
\end{notation}

\begin{defn}
Formulas $x \realize A$ are defined by induction
on the structure of $A$:
%\footnotesize
\begin{align*}
\Lambda \realize A &:= A \ \ \ (A \text{ atomic}) \\
\mathbf{x}, \mathbf{y} \realize (B\wedge C)
&:=
(\mathbf{x} \realize B) \wedge (\mathbf{y} \realize C) \\
z, \mathbf{x}, \mathbf{y} \realize
(B\vee C) &:=
(z= \zeroT \wedge \mathbf{x} \realize B) \vee
(z \neq \zeroT \wedge \mathbf{y} \realize C) \\
\mathbf{y} \realize (B\rightarrow C) &:=
\forall \mathbf{x}.((\mathbf{x} \realize B)
\rightarrow \mathbf{y}(\mathbf{x}) \realize C)
\wedge (B\rightarrow C) \\
z,\mathbf{x} \realize \exists y.B &:=
\mathbf{x} \realize B\{z/y\} \\
\mathbf{x} \realize \forall y.B &:=
\forall y.(\mathbf{x}(y) \realize B),
\end{align*}
\normalsize
where no variable in $\mathbf{x}$ occurs free in $A$.
Given terms $\mathbf{t} = \tTerm_1,\dots, \tTerm_n$,
$
\mathbf{t} \realize A := (\mathbf{x} \realize A) \{\mathbf{t}/\mathbf{x}\}.
$
\end{defn}
\noindent
We can now link derivability of such formulas
with that of formulas in $I\POR^\lambda$.

%%% SOUNDNESS AND COMPLETENESS
\begin{theorem}[Soundness and Completeness]\label{thm:completeness}
\begin{itemize}
\itemsep0em
\item[i]
If $\vdash_{I\POR^\lambda} \mathbf{t} \realize A$,
then $\vdash_{I\POR^\lambda} A$.
\item[ii.] If $\vdash_{I\POR^\lambda} A$,
then there exist $\mathbf{t}$ such that $\vdash_{I\POR^\lambda}
\mathbf{t}\realize A$.
\end{itemize}
\end{theorem}
\begin{proof}[Proof Sketch]
Proofs are by induction on formulas
($i.$) and on derivation height ($ii.$).
\end{proof}

%%% COROLLLARY 3
\begin{cor}\label{cor3}
Let $\forall x.\exists y.A(x,y)$
be a closed theorem of $I\POR^\lambda$,
where $A$ is a $\Sigma^b_1$-formula.
Then, there is a closed term $\tTerm:\sType \arrowT
\sType$ of $\POR^\lambda$, such that:
$\vdash_{I\POR^\lambda}(\forall x)A(x,\tTerm x)$
\end{cor}
\begin{proof}
By Theorem~\ref{thm:completeness}$.ii$,
there is $\mathbf{w}=\tTerm,w$ such that
$\vdash_{I\POR^\lambda} \mathbf{w} \realize (\forall x)(\exists y)A(x,y)$,
\begin{align*}
\mathbf{w} \realize (\forall x)(\exists y)A(x,y)
&\equiv
(\forall x)(\mathbf{w}(x) \realize (\exists y)A(x,y)) \\
&\equiv
(\forall x)(w(x) \realize A(x,\tTerm x)).
\end{align*}
From this, by Theorem~\ref{thm:completeness}$.i$,
we conclude
$\vdash_{I\POR^\lambda} \forall x.A(x,\tTerm x)$.
\end{proof}
We can now prove
that if a function is $\Sigma^b_1$-representable
in $I\RS$, then it is in $\POR$.
\begin{cor}\label{cor4}
For any function $f:\Os \times \Ss \rightarrow \Ss$,
if there is a closed $\Sigma^b_1$-formula $A(x,y)$
in $\Lpw$ such that
(1) $I\RS \vdash \forall x.\exists !y.A(x,y)$,
(2) $\model{A(\ooverline{s_1},\ooverline{s_2})} = \{\omega
\ | \ f(\omega, s_1)=s_2\}$,
then $f\in\POR$.
\end{cor}
\begin{proof}
Since $\vdash_{I\RS} \forall x.\exists !y.A(x,y)$,
by Theorem~\ref{theorem2},
also $\vdash_{I\POR}\forall x.\exists !y.A(x,y)$,
from which we deduce
$\vdash_{I\POR^\lambda} \forall x.A(x,\gTerm x)$
for some closed term $\gTerm : \sType \arrowT
\sType$ of $\POR^\lambda$, by Cor~\ref{cor3}
and by Theorem~\ref{theorem1},
there is a function $g\in \POR$ such that for any
$\omega \in \Os$ and $s_1,s_2\in \Ss$,
$
T_\omega \vdash_{I\POR^\lambda} A(\ooverline{s_1},
\ooverline{s_2}) \Leftrightarrow g(s_1,\omega)=s_2.
$
From this we conclude,
\begin{align*}
g(s_1,\omega= s_2) \ \ \ &\Leftrightarrow \ \ \
T_\omega \vdash_{I\POR^\lambda} A(\ooverline{s_1},
\ooverline{s_2}) \\
&\Leftrightarrow \ \ \ \omega \in \model{A(\ooverline{s_1},
\ooverline{s_2})} \\
&\Leftrightarrow \ \ \ f(s_1,\omega) = s_2.
\end{align*}
So, since $f=g$, we conclude that $f\in \POR$.
\end{proof}

\paragraph*{Concluding the Proof}
To conclude we need to extend
Corollary~\ref{cor4} to classical $\RS$,
showing that any function which is $\Sigma^b_1$-representable
in $\RS$ is also in $\POR$.
%
%The proof is obtained by adapting the method  from~\cite{CookUrqhuart}.
%
%To do so,
We start by generalizing $I\POR^\lambda$
via EM, $A\vee \neg A$.
We show that realizability interpretation
extends to such $I\POR^\lambda$+EM,
so that for any of its closed theorems
$\forall x.\exists y\preceq \tTerm. A(x,y)$,
with $A\in \Sigma^b_1$, there is a closed term
$\tTerm : \sType \arrowT \sType$ of $\POR^\lambda$,
such that $\vdash_{I\POR^\lambda}\forall x.A(x,\tTerm x)$.
To do so, we pass through Markov's principle.

%%% Markov's Principle
\begin{defn}[Markov's Principle]
For any $A\in \Sigma^b_1$,
Markov's principle is defined as:
\begin{align}
\neg \neg \exists x.A \rightarrow \exists x.A.
\tag{Markov}
\end{align}
\end{defn}

\begin{prop}\label{prop5}
For any $\Sigma^b_1$-formula $A$,
if $\vdash_{I\POR^\lambda + EM} A$, then
$\vdash_{I\POR^\lambda + (Markov)} A$.
\end{prop}
\begin{proof}[Proof Sketch]
The proof relies on double-negation translation.
Notice that for any $\Sigma^b_0$-formula $A$,
$\vdash_{I\POR^\lambda} \neg \neg A \rightarrow A$.
\end{proof}
\noindent
Now, we need to show that the realizability
interpretation extends to $I\POR^\lambda$+(Markov),
that is for any of its closed theorems
$\forall x.\exists y \preceq \tTerm.A(x,y)$,
with $A \in \Sigma^b_1$, there is a closed term
$\tTerm : \sType \arrowT \sType$
of $\POR^\lambda$, such that
$\vdash_{I\POR^\lambda} \forall x.A(x,\tTerm x)$.
Then, given a subjective encoding
$\sharp : (\sType \arrowT \sType) \arrowT \sType$
in $I\POR^\lambda$ of first-order unary functions
as strings, together with a ``decoding'' function
$\app: \sType \arrowT \sType \arrowT \sType$
satisfying $\vdash_{I\POR^\lambda} \app(\sharp \fTerm,x)
=\fTerm x$.
Moreover, let
\begin{align*}
x* y &:= \sharp(\lambda z.\BAnd (\app(x,z), \app(y,z))) \\
T(x) &:= \exists y.\BT(\app(x,y))=\zeroT.
\end{align*}
There is a \emph{meet semi-lattice} structure
on the set of terms of type $\sType$ defined
by $\tTerm \sqsubseteq \uTerm$
iff $\vdash_{I\POR^\lambda} T(\uTerm) \rightarrow
T(\tTerm)$ with top element $\underline{\oone} =\sharp(\lambda x.\oneT)$
and meet given by $x*y$.
Indeed, from $T(x*\oneT) \leftrightarrow T(x)$,
$x\sqsubseteq \underline{\oone}$
follows.
Moreover, from $\BT(\app(x,\uTerm))=\zeroT$,
we obtain $\BT(\app(x*y,\uTerm))=\BAnd(\app(x,\uTerm),\app(y,\uTerm))=\zeroT$,
whence $T(x) \rightarrow T(x*y)$,
i.e.~$x*y \sqsubseteq x$.
In a similar way, we prove $x*y\sqsubseteq y$.
Finally, from $T(x)\rightarrow T(v)$
and $T(y)\rightarrow T(v)$,
we deduce $T(x*y) \rightarrow T(v)$,
observing that $\vdash_{I\POR^\lambda} T(x*y) \rightarrow
T(y)$.
Notice that the formula $T(x)$
is \emph{not} in $\Sigma^b_1$,
as its existential quantifier is not bounded.

\begin{defn}
For any formula $A$ of $I\POR^\lambda$
and fresh variable $x$, we define $x\Vdash A$:
%\footnotesize
\begin{align*}
x \Vdash A &:= A \vee T(x) \ \ \ \ (A \text{ atomic}) \\
x \Vdash B \triangleright C &:= x \Vdash B \triangleright x \Vdash C \\
x \Vdash B\rightarrow C &:= \forall y(y \vDash B
\rightarrow x*y\vDash X) \\
x \Vdash \mathscr{Q}y.B &:= \mathscr{Q}y. x \Vdash B.
\end{align*}
\normalsize
where $\triangleright \in \{\vee,\wedge\}$,
and $\mathscr{Q}\in\{\exists, \forall\}$.
\end{defn}

The following Lemma~\ref{lemma3} is proved by
induction on the structure of formulas,
together with a series of intermediate results.

\begin{lemma}\label{lemma3}
If $\vdash_{I\POR^\lambda} A$ without using
$\NP$-induction,
then
$\vdash_{I\POR^\lambda} x\vDash A$.
\end{lemma}

\begin{lemma}\label{lemma10}
Let $A=\exists x\preceq \tTerm.B$,
where $B \in \Sigma^b_0$.
Then, there is a term $\uTerm:\sType$,
with FV($\uTerm_A)$=FV($B$) such that
$\vdash_{I\POR^\lambda} A \leftrightarrow T(\uTerm_A)$.
\end{lemma}
From which we deduce the following three properties
for any $A\in \Sigma^b_1$:
\begin{enumerate}
\itemsep0em
\item[i.] $\vdash_{I\POR^\lambda} (x\Vdash A) \leftrightarrow
(A\vee T(x))$
\item[ii.] $\vdash_{I\POR^\lambda} (x\Vdash \neg A)
\leftrightarrow (A\rightarrow T(x))$
\item[iii.] $\vdash_{I\POR^\lambda} (x\Vdash \neg\neg A)
\leftrightarrow (A\vee T(x))$,
\end{enumerate}

\begin{cor}[Markov]
If $A$ is a $\Sigma^b_1$-formula,
then $\vdash_{I\POR^\lambda} x \Vdash \neg \neg A
\rightarrow A$.
\end{cor}

Finally, we define the extension $(I\POR^\lambda)^*$
of $I\POR$, using PIND.

\begin{defn}[PIND]
Let PIND$(A)$ indicate the formula:
$$
(A(\epsilonT) \wedge (\forall x.(A(x)
\rightarrow A(x\zeroT)) \wedge
\forall x.(A(x) \rightarrow A(x\oneT)) \rightarrow
\forall x.A(x).
$$
\end{defn}
Observe that if $A(x)$ is in the form
$\exists y \preceq \tTerm.\uTerm = \vTerm$,
then the formula $z\Vdash$ PIND$(A)$
is of the form PIND$(A(x) \vee T(z))$,
which is \emph{not} an instance of the
$\NP$-induction schema (as $T(z)= \exists x.\BT(\app(z,x))=\zeroT$ is not bounded).

\begin{defn}[Theory $(I\POR^\lambda)^*$]
Let $(I\POR^\lambda)^*$ indicate the theory
extending $I\POR^\lambda$ with all instances of the induction schema PIND$(A(x)\vee B)$,
where $A(x)$ is of the form $\exists y\preceq \tTerm.
\uTerm=\vTerm$ and $B$ is an arbitrary formula with
$x\not\in$ FV$(B)$.
\end{defn}

\begin{prop}
For any $\Sigma^b_1$-formula $A$,
if $\vdash_{I\POR^\lambda} A$,
then $\vdash_{(I\POR^\lambda)^*} x \Vdash A$.
\end{prop}
We can also extend the realizability interpretation
to $(I\POR^\lambda)^*$ by simply constructing
a realizer for PIND$(A(x) \vee B)$.

\begin{lemma}\label{lemma4}
Let $A(x):=\exists y\preceq \tTerm.\uTerm=\zeroT$
and $B$ be any formula not containing free occurrences
of $x$.
Then, there exist $\mathbf{t}$ such that
$\vdash_{I\POR^\lambda} \mathbf{t} \realize PIND(A(x) \vee B)$.
\end{lemma}
So, by Theorem~\ref{thm:completeness}$.i$,
we observe that for any $\Sigma^b_1$-formula
$A$ and $B$ with $x\not\in$ FV$(A)$,
$\vdash_{I\POR^\lambda}$ PIND$(A(x)\vee B)$.

\begin{cor}%[$\forall \NP$-Conservativity of $I\POR^\lambda$ + EM over $I\POR^\lambda$]
For $A\in \Sigma^b_1$,
if $\vdash_{I\POR^\lambda + EM} \forall x.\exists y\preceq \tTerm. A(x,y)$, then
$\vdash_{I\POR^\lambda} \forall x.\exists y\preceq \tTerm.
A(x,y)$.
\end{cor}

We conclude by proving the Prop.~\ref{prop6}
below:
\begin{prop}\label{prop6}
Let $\forall x.\exists y\preceq \tTerm.A(x,y)$
be a closed theorem of $I\POR^\lambda$ + (Markov),
with $A\in\Sigma^b_1$.
Then, there is a $\tTerm:\sType \arrowT \sType$
of $\POR^\lambda$ such that
$\vdash_{I\POR^\lambda} \forall x.A(x,\tTerm x)$.
\end{prop}
\begin{proof}
If $I\POR^\lambda$ + (Markov) proves $\forall x.\exists y.
A(x,y)$, then by Prop~\ref{prop:Parikh}
it also proves $\exists y\preceq \tTerm.A(x,y)$
and $\vdash_{(I\POR)^*} z\Vdash \exists y\preceq \tTerm.
A(x,y)$.
Let $B:= \exists y \preceq \tTerm.A(x,y)$
and $\zTerm=\uTerm_C$, by Lemma~\ref{lemma4},
$\vdash_{(I\POR^\lambda)^*} B$ and so,
by Lemma~\ref{lemma3} and~\ref{lemma10},
we conclude that there are $\mathbf{t},\mathbf{u}$
such that $\vdash_{I\POR^\lambda} \mathbf{t},
\mathbf{u} \realize B$,
which implies $\vdash_{I\POR^\lambda}A(x,\mathbf{t} x)$.
Thus, $\vdash_{I\POR^\lambda} \forall x.A(x), \mathbf{t} x$.
\end{proof}

So by Prop~\ref{prop5},
if $\vdash_{I\POR^\lambda + EM}\forall x.\exists \preceq \tTerm.A(x,y)$, where $A$ is a closed $\Sigma^b_1$-formula,
then there is a closed term $\tTerm:\sType \arrowT \sType$
of $\POR^\lambda$ such that
$\vdash_{I\POR^\lambda} \forall x.A(x,\tTerm x)$.
As for Corollary~\ref{cor4},

\begin{cor}
Let $\RS \vdash \forall x.\exists y\preceq \tTerm.A(x,y)$,
where $A$ is a $\Sigma^b_1$-formula with only
$x,y$ free.
For any function $f:\Ss\times \Os \rightarrow \Ss$,
if $\forall x.\exists y \preceq \tTerm.A(x,y)$ represents $f$
so that (1) $\RS \vdash \forall x.\exists ! y.A(x,y)$,
(2) $\model{A(\ooverline{s_1},\ooverline{s_2}}=
\{\omega \ | \ f(s_1,\omega)=s_2\}$,
then $f\in \POR$.
\end{cor}
